# Supplementary material for: Streaming quanta sensors for online, high-performance imaging and vision
Source: arXiv:2406.00859 source file (2024-06-02)
Supplement: Supplementary file 1 [file supp.tex]

\ifCLASSINFOpdf
  % \usepackage[pdftex]{graphicx}
  % declare the path(s) where your graphic files are
  % \graphicspath{{../pdf/}{../jpeg/}}
  % and their extensions so you won't have to specify these with
  % every instance of \includegraphics
  % \DeclareGraphicsExtensions{.pdf,.jpeg,.png}
\else
  % or other class option (dvipsone, dvipdf, if not using dvips). graphicx
  % will default to the driver specified in the system graphics.cfg if no
  % driver is specified.
  % \usepackage[dvips]{graphicx}
  % declare the path(s) where your graphic files are
  % \graphicspath{{../eps/}}
  % and their extensions so you won't have to specify these with
  % every instance of \includegraphics
  % \DeclareGraphicsExtensions{.eps}
\fi
\maketitle

\IEEEdisplaynontitleabstractindextext

\IEEEpeerreviewmaketitle

\section{Detailed Information about dataset generation}
\subsection{NFS dataset}
RIFE produces high-quality interpolations, as long as the original video (to be interpolated) is largely free of noise and blur. Note that here, the interpolation must be done recursively multiple times -- each time with an interpolation factor of 2x or 4x, as direct 16x interpolation introduces visual artifacts. After interpolation, we spatially downsample the videos by 2x to reduce the downstream effects of any remnant interpolation artifacts (caused by any slight blur and compression). Finally, each video generated through is process is manually inspected and any video segments with visible interpolation artifacts are removed from the dataset. The frames are then converted to grayscale and ready to use. The NFS dataset mostly contains global camera motion and some local object motion sequences. We produced around 50 long sequences in total using this procedure. One key benefit of the NFS dataset is that it contains many long hundred-frame or thousand-frame videos. This duration is very suitable for producing training data for our context as thousands of binary frames are needed to generate one training sample. 

\subsection{Kubric local motion dataset}
We use Kubric, a scalable Python-based simulator, for rendering synthetic videos \cite{greff2022kubric} with local motion. We program the motion of foreground objects in front of a static background. For the foreground objects, we randomly draw samples from ShapeNet assets \cite{chang2015shapenet}. Raw images from the RAISE raw dataset \cite{dang2015raise} are used as static background. In totality, we simulated about 40 long sequences, each with a length of 25000 frames, with a rendering resolution of 300x300. Half of the sequences contain object rotation, and the other half contain translation. For translation, we generate trajectories roughly in the FOV that are either piecewise linear or piecewise Bezier (with one random control point per segment, and 5-10 segments in total per sequence). For each linear segment, the endpoints are randomly sampled within a unit sphere that lies largely in the FOV of the camera. For rotation, we perform similar sampling operations in rotational coordinate space. 

The motion sequence set covers a wide range of velocities, objects, occlusions, and motion scenarios, encompassing global and local motions. The fine-grained motion is suitable for mimicking underlying intensities at the operation speed of high-speed QIS (0–10000 pixels/s). This diverse dataset is crucial for effectively training the reconstruction network. Additionally, our methods can be adapted for specific cases required in future studies. For instance, one can capture a slow-moving global motion dataset using a mobile phone, and interpolate the videos to generate ground truth reference frames at 10 kFPS, given that there is no blur in the hand motion and the interpolation factor aligns with the correct interframe motion range. 

\bibliographystyle{IEEEtran}
\bibliography{references}
